# Supplementary material for: Style is NOT a single variable: Case Studies for Cross-Style Language Understanding
Source: arXiv:1911.03663 source file (2021-06-02)
Supplement: Supplementary file 1 [file additional.tex]

% % \section{Cross-Style Stylistic Generation: Snapshot}
% % \begin{figure*}[ht!]
% % \vspace{0mm}
% % \centering
% % {
% % \includegraphics[trim=0cm 0cm 2cm  0cm,clip,width=.99\linewidth]{figs/{generation_snapshot}.pdf}
% % }
% % \caption{\label{fig:cross_style_generation} Demonstration of our cross-style text synthesizer. A simple workflow of our demo is as follows: (0) type or choose a text, (1) tsynthesize the input text: predicts multiple style values given the text, and (2) control the style value by moving the sliding bar: a new stylized text appear at the bottom.   }
% % \vspace{0mm}
% % \end{figure*}




% % \section{Discussion with Ed}
% % Intuitively, as you point out, there seem to be a lot of sensible predictions.  However with precisely this sort of thing, and with such a bold paper, one has to be super-careful with the statistics.  So the main thing I was looking for, and that I think definitely is required here, are some internal correlation and also validity/significance scores.  I can easily imagine people objecting that these 'styles’ are not precisely defined, and that they overlap/correlate, so it is unclear how many independent things one is working with.  (This is, of course, a core problem with stylistic analysis, so it is therefore all the more reason to be extra-careful.) 


% % Fortunately, Taehee should know about Analysis of Covariance (see for example the ANCOVA article in Wikipedia at \url{https://en.wikipedia.org/wiki/Analysis_of_covariance)}. It would be nice to build a general plan/script for how to show which of these variables are truly independent of one another, and incidentally how that correlates (it should I suppose) with the clustering dendrogram.  Then you will have two (or more) independent algorithms for showing style factor covariance — ANCOVA and classification (using various source algorithms).  And the overall argument will be: 
% % - we define textual phenomena A and B and C … 
% % - we run various NLP classifiers for each phenomenon 
% % - we discover the classifications co-vary in many cases 
% % - we also run ANCOVA (and appropriate variations) 
% % - we discover the same, with stat significance 
% % - so, we conclude, that certain phenomena co-vary 
% % - these co-varying clusters are what we call Style (with a capital S); each S consists of a bunch of semi-independent phenomena that conspire together to create their S 
% % - here are some examples 

% % Once the statistics is formally settled, the objections move one level ‘down’, namely to the nature/definition of each individual phenomenon.  I[ can’t bring myself to call them ’styles' because, to me, the phenomena are a mixture of a lot of types of things.  Some of them are in fact styles (in the sense I understand it), but others are not.  But their co-varying combinations are exactly what I think of as ’style’ in its normal sense.]  Here the paper does not have space to define these phenomena adequately —that has to go into the thesis— bt it should give e some idea (as you do now) and point to the thesis, where the definitive definitions and analyses and corpora are described.  

% % I think it might also be a safeguard to state somewhere, carefully, that it is probably impossible to define _exactly_ what makes any individual phenomenon, but we are in general dealing with word usage preferences in regular groups, and we assign suggestive names to these groups insofar as we can think of them and assemble a corpus.  So it is easy to assemble a collection of text with feature X, where X = “written by people between 35 and 45” or X = “written by people who were in the war in Vietnam” r X = “written by people who have dark-brown hair”, and we discover analytically that some of these collections share some word usage patterns that statistically vary with other contracting groups X1, X2, etc., while others do not.  So “written by people who were in the war in Korea” may be an X1, and “written by people with blonde hair” may be another, and weight find a statistically significant variation between X and X1 for the war grouping but nothing for the hair color grouping.  In that way, we analytically discover phenomena that become the building blocks of style.  (And indeed, perhaps one can say these phenomena, so discovered, are styles themselves, as you call them.  I have to think about that.) 

% % # risk of making bold and (probably) over-claiming statements on the ethical subjects (especially, certain groups of persona)
% % I think I have to be very careful to make any claims related to specific groups of people and their language styles. For example, making a claim like “people only with high school education likely speak informal language” might be ethically risky and statistically wrong. We should rather say that “there is a X.XX% of positive correlation between text written by one with high-school education and text which is predicted as information by our classifiers” where the correlation is derived from ANCOVA.  

% % # definition of styles
% % I guess you already realize that I prefer to call the high-level categories of language usage (e.g., metaphor, sentiment, personas) as styles in a broader sense, while your definition of style is somewhat more internal phenomenon of linguistic features (e.g., lexical, syntactic) that actually caused or are caused by the text variation. Here is a reason of why I still like to call the former as "styles" and the latter as " features in stylistic text variation". In my perspective, people often use the broader definition of style here and there so it might be better to use same terminology (?), although they have wrong understanding of what style is. Even worse thing is that they don't look at how the internal features matter in the variation at all, instead they just hope neural models deal with it somehow. You can imagine that all the recent style-transfer papers never care about what features are used in the variation. 

% % However, this paper is not intended to explore the internal phenomenon across styles yet rather only focuses on suggesting a new research direction; cross-style language understanding, with some of its potential applications and analyses. Shirley and Taehee are looking into more in-depth statistical analysis (i.e., pair-plot, causality) on the cross-style behavior and its coupled-ness to semantics of text, which is called “style dynamics” (i.e.., some text is stylistically dynamic and changeable, while other is not). 

% % Another separate paper should follow is the generation paper by training (cross-style) text generation models on the set of datasets collected and studying how different features (e.g., words, pronoun usage, sentence length) are used across styles in terms of generation.

% % Getting back to this paper, as you said, I will make a clear distinction between the category of stylistic language and the features related to the text variation, and make the clear point of my definition of style and its scope. Also, I will point out how difficult to make exact scope/definition of styles in general and how difficult to find what features make individual phenomenon, particularly in cross-style setting.

% % # case study 
% % I like the idea of making (in)dependent set of text groups with their actual grouping labels for the sake of validation. I will try a simple experiment on this.

% % # covariance analysis
% % I always forget your lesson on this (i.e., statistical significance) since I am little rushed to get the results at the end :) (Un)fortunately, you are not the one who complains about it. Taehee also always points about the lack of statistical evidence of my work, too :-( I will add the better covariance analysis in the paper! Thank you for the reminder again. 


% \begin{figure*}[ht!]
% \vspace{0mm}
% \centering
% {
% \includegraphics[trim=0cm 0cm 0cm  0cm,clip,width=.99\linewidth]{figs/{corr_cluster=False_limit=100_multi_3}.png}
% }
% \caption{\label{fig:style_corr_more} Correlation analysis on different styles. Best viewed in color. }
% \vspace{0mm}
% \end{figure*}
